# Supplementary material for: DeepNcode: Encoding-Based Protection against Bit-Flip Attacks on Neural Networks
Source: arXiv:2405.13891 source file (2024-06-02)
Supplement: Supplementary file 1 [file appendix.tex]

\begin{table*}
    \centering
    \scalebox{1}{
    \begin{tabular}{|c|c|c|c|c|c|}\cline{4-6}
        \multicolumn{3}{c|}{} & \multicolumn{3}{c|}{Attack success rate $(\%)$} \\\hline
        Dataset & Attack & Model & avg & min & max \\\hline
        \parbox[t]{2mm}{\multirow{10}{*}{\rotatebox[origin=c]{90}{CIFAR-10}}} & \multirow{2}{*}{BFA} & ResNet-20 & $ 100.0 \pm 0.00 $ & 100.0 & 100.0 \\
                                                                                                 &    & VGG-11 & $ 100.0 \pm 0.00 $ & 100.0 & 100.0  \\\cline{2-6}
                                                                            & \multirow{2}{*}{\makecell{T-BFA\\ \textit{N-to-1}}} & ResNet-20 & $ 100.0 \pm 0.00 $ & 100.0 & 100.0 \\
                                                                                                 &    & VGG-11  & $ 100.0 \pm 0.00 $ & 100.0 & 100.0 \\\cline{2-6}
                                                                             & \multirow{2}{*}{\makecell{T-BFA\\ \textit{1-to-1}}} & ResNet-20 & $ 99.95 \pm 0.15 $ & 99.0 & 100.0 \\
                                                                                                 &    & VGG-11 & $ 99.97 \pm 0.10 $ & 99.40 & 100.0 \\\cline{2-6}
                                                                             & \multirow{2}{*}{\makecell{T-BFA\\ \textit{1-to-1 stealthy}}} & ResNet-20 & $ 98.26 \pm 1.15 $ & 95.0 & 100.0 \\
                                                                                                 &    & VGG-11 & $ 47.04 \pm 47.56 $ & 0.0 & 99.0 \\\cline{2-6}
                                                                            & \multirow{2}{*}{TA-LBF} & ResNet-20 & $ 100.0 \pm 0.00 $ & 100.0 & 100.0 \\
                                                                                                 &    & VGG-11 & $ 100.0 \pm 0.00 $ & 100.0 & 100.0\\\hline\hline
       \parbox[t]{2mm}{\multirow{10}{*}{\rotatebox[origin=c]{90}{CIFAR-100}}} & \multirow{2}{*}{BFA} & ResNet-18 & $ 100.0 \pm 0.00 $ & 100.0 & 100.0 \\
                                                                                                 &    & VGG-11 & $ 100.0 \pm 0.00 $ & 100.0 & 100.0 \\\cline{2-6}
                                                                            & \multirow{2}{*}{\makecell{T-BFA\\ \textit{N-to-1}}} & ResNet-18 & $ 100.0 \pm 0.00 $ & 100.0 & 100.0 \\
                                                                                                 &    & VGG-11 & $ 100.0 \pm 0.004 $ & 99.98 & 100.0 \\\cline{2-6}
                                                                             & \multirow{2}{*}{\makecell{T-BFA\\ \textit{1-to-1}}} & ResNet-18 & $ 99.92 \pm 0.63 $ & 94.0 & 100.0 \\
                                                                                                 &    & VGG-11 & $ 99.92 \pm 0.63 $ & 94.0 & 100.0 \\\cline{2-6}
                                                                             & \multirow{2}{*}{\makecell{T-BFA\\ \textit{1-to-1 stealthy}}} & ResNet-18  & $ 9.52 \pm 27.96 $ & 0.0 & 100.0 \\
                                                                                                 &    & VGG-11 & $ 1.6 \pm 5.24 $ & 0.0 & 36.0 \\\cline{2-6}
                                                                            & \multirow{2}{*}{TA-LBF} & ResNet-18 & $ 100.0 \pm 0.00 $ & 100.0 & 100.0 \\
                                                                                                 &    & VGG-11 & $ 100.0 \pm 0.00 $ & 100.0 & 100.0 \\\hline                                                                                       
    \end{tabular}}
    \vspace{3mm}
    \caption{$4-$bit T-BFA from Attack sample}
\end{table*}

\begin{table*}
    \centering
    \scalebox{1}{
    \begin{tabular}{|c|c|c|c|c|c|}\cline{4-6}
        \multicolumn{3}{c|}{} & \multicolumn{3}{c|}{Attack success rate $(\%)$} \\\hline
        Dataset & Attack & Model & avg & min & max \\\hline
        \parbox[t]{2mm}{\multirow{10}{*}{\rotatebox[origin=c]{90}{CIFAR-10}}} & \multirow{2}{*}{BFA} & ResNet-20 & $ 100.0 \pm 0.00 $ & 100.0 & 100.0 \\
                                                                                                 &    & VGG-11 & $ 100.0 \pm 0.00 $ & 100.0 & 100.0  \\\cline{2-6}
                                                                            & \multirow{2}{*}{\makecell{T-BFA\\ \textit{N-to-1}}} & ResNet-20 & $ 100.0 \pm 0.00 $ & 100.0 & 100.0 \\
                                                                                                 &    & VGG-11  & $ 100.0 \pm 0.003 $ & 99.98 & 100.0 \\\cline{2-6}
                                                                             & \multirow{2}{*}{\makecell{T-BFA\\ \textit{1-to-1}}} & ResNet-20  & $ 99.94 \pm 0.21 $ & 98.20 & 100.0 \\
                                                                                                 &    & VGG-11 & $ 99.98 \pm 0.08 $ & 99.40 & 100.0 \\\cline{2-6}
                                                                             & \multirow{2}{*}{\makecell{T-BFA\\ \textit{1-to-1 stealthy}}} & ResNet-20 & $ 98.08 \pm 0.94 $ & 95.60 & 100.0 \\
                                                                                                 &    & VGG-11& $ 5.86 \pm 19.68 $ & 0.0 & 91.20 \\\cline{2-6}
                                                                            & \multirow{2}{*}{TA-LBF} & ResNet-20 & $ 100.0 \pm 0.00 $ & 100.0 & 100.0 \\
                                                                                                 &    & VGG-11 & $ 100.0 \pm 0.00 $ & 100.0 & 100.0 \\\hline\hline
       \parbox[t]{2mm}{\multirow{10}{*}{\rotatebox[origin=c]{90}{CIFAR-100}}} & \multirow{2}{*}{BFA} & ResNet-18 & $ 100.0 \pm 0.00 $ & 100.0 & 100.0 \\
                                                                                                 &    & VGG-11 & $ 100.0 \pm 0.00 $ & 100.0 & 100.0 \\\cline{2-6}
                                                                            & \multirow{2}{*}{\makecell{T-BFA\\ \textit{N-to-1}}} & ResNet-18 & $ 100.0 \pm 0.00 $ & 100.0 & 100.0 \\
                                                                                                 &    & VGG-11 & $ 100.0 \pm 0.004 $ & 99.98 & 100.0 \\\cline{2-6}
                                                                             & \multirow{2}{*}{\makecell{T-BFA\\ \textit{1-to-1}}} & ResNet-18 & $ 99.84 \pm 0.83 $ & 94.0 & 100.0 \\
                                                                                                 &    & VGG-11& $ 99.44 \pm 1.60 $ & 90.0 & 100.0 \\\cline{2-6}
                                                                             & \multirow{2}{*}{\makecell{T-BFA\\ \textit{1-to-1 stealthy}}} & ResNet-18  & $ 5.86 \pm 21.59 $ & 0.0 & 100.0 \\
                                                                                                 &    & VGG-11 & $ 0.54 \pm 1.41 $ & 0.0 & 8.0 \\\cline{2-6}
                                                                            & \multirow{2}{*}{TA-LBF} & ResNet-18 & $ 100.0 \pm 0.00 $ & 100.0 & 100.0 \\
                                                                                                 &    & VGG-11 & & & \\\hline                                                                                       
    \end{tabular}}
    \vspace{3mm}
    \caption{$8-$bit T-BFA from Attack sample}
\end{table*}

\begin{table*}
    \centering
    \scalebox{1}{
    \begin{tabular}{|c|c|c|c|c|c|}\cline{4-6}
        \multicolumn{3}{c|}{} & \multicolumn{3}{c|}{Attack success rate $(\%)$} \\\hline
        Dataset & Attack & Model & avg & min & max \\\hline
        \parbox[t]{2mm}{\multirow{4}{*}{\rotatebox[origin=c]{90}{CIFAR-10}}} 
                                                                             & \multirow{2}{*}{\makecell{T-BFA\\ \textit{1-to-1}}} & ResNet-20 & $ 100.0 \pm 0.00 $ & 100.0 & 100.0 \\
                                                                                                 &    & VGG-11 & $ 100.0 \pm 0.00 $ & 100.0 & 100.0 \\\cline{2-6}
                                                                             & \multirow{2}{*}{\makecell{T-BFA\\ \textit{1-to-1 stealthy}}} & ResNet-20 & $ 97.50 \pm 1.29 $ & 93.0 & 99.40 \\
                                                                                                 &    & VGG-11 & $ 46.86 \pm 47.41 $ & 0.0 & 98.60
                                                                             \\\hline\hline
       \parbox[t]{2mm}{\multirow{4}{*}{\rotatebox[origin=c]{90}{CIFAR-100}}}
                                                                             & \multirow{2}{*}{\makecell{T-BFA\\ \textit{1-to-1}}} & ResNet-18 & $ 100.0 \pm 0.00 $ & 100.0 & 100.0 \\
                                                                                                 &    & VGG-11 & $ 99.74 \pm 0.92 $ & 94.0 & 100.0 \\\cline{2-6}
                                                                             & \multirow{2}{*}{\makecell{T-BFA\\ \textit{1-to-1 stealthy}}} & ResNet-18  & $ 8.66 \pm 26.40 $ & 0.0 & 100.0 \\
                                                                                                 &    & VGG-11 & $ 0.96 \pm 3.46 $ & 0.0 & 28.0 \\\hline                                                                                       
    \end{tabular}}
    \vspace{3mm}
    \caption{$4-$bit T-BFA from rest of the source class}
\end{table*}

\begin{table*}
    \centering
    \scalebox{1}{
    \begin{tabular}{|c|c|c|c|c|c|}\cline{4-6}
        \multicolumn{3}{c|}{} & \multicolumn{3}{c|}{Attack success rate $(\%)$} \\\hline
        Dataset & Attack & Model & avg & min & max \\\hline
        \parbox[t]{2mm}{\multirow{4}{*}{\rotatebox[origin=c]{90}{CIFAR-10}}} 
                                                                            & \multirow{2}{*}{\makecell{T-BFA\\ \textit{1-to-1}}} & ResNet-20  & $ 100.0 \pm 0.00 $ & 100.0 & 100.0 \\
                                                                                                 &    & VGG-11 & $ 100.0 \pm 0.02 $ & 99.80& 100.0 \\\cline{2-6}
                                                                             & \multirow{2}{*}{\makecell{T-BFA\\ \textit{1-to-1 stealthy}}} & ResNet-20 & $ 97.51 \pm 1.06 $ & 94.80 & 99.80 \\
                                                                                                 &    & VGG-11& $ 5.83 \pm 19.71 $ & 0.0 & 89.60 
                                                                            \\\hline\hline
       \parbox[t]{2mm}{\multirow{4}{*}{\rotatebox[origin=c]{90}{CIFAR-100}}} 
                                                                             & \multirow{2}{*}{\makecell{T-BFA\\ \textit{1-to-1}}} & ResNet-18 &  $ 100.0 \pm 0.00 $ & 100.0 & 100.0 \\
                                                                                                 &    & VGG-11& $ 99.84 \pm 0.73 $ & 96.0 & 100.0 \\\cline{2-6}
                                                                             & \multirow{2}{*}{\makecell{T-BFA\\ \textit{1-to-1 stealthy}}} & ResNet-18  & $ 5.72 \pm 20.96 $ & 0.0 & 100.0 \\
                                                                                                 &    & VGG-11 & $ 0.52 \pm 1.59 $ & 0.0 & 12.0 
                                                                            \\\hline                                                                                       
    \end{tabular}}
    \vspace{3mm}
    \caption{$8-$bit T-BFA from rest of the source class}
\end{table*}

\begin{table*}
    \centering
    \scalebox{1}{
    \begin{tabular}{|c|c|c|c|c|c|}\cline{4-6}
        \multicolumn{3}{c|}{} & \multicolumn{3}{c|}{Post attack accuracy $(\%)$} \\\hline
        Dataset & Precision & Model & avg & min & max \\\hline
        \parbox[t]{2mm}{\multirow{4}{*}{\rotatebox[origin=c]{90}{CIFAR-10}}} 
                                                                            & \multirow{2}{*}{4-bit} & ResNet-20  & $ 84.96 \pm 5.48 $ & 56.85 & 91.48 \\
                                                                                                 &    & VGG-11 & $ 90.91 \pm 0.73 $ & 88.73 & 92.76 \\\cline{2-6}
                                                                             & \multirow{2}{*}{8-bit} & ResNet-20 & $ 85.13 \pm 6.82 $ & 45.68 & 90.78 \\
                                                                                                 &    & VGG-11& $ 89.90 \pm 8.00 $ & 39.87 & 93.92
                                                                            \\\hline\hline
       \parbox[t]{2mm}{\multirow{4}{*}{\rotatebox[origin=c]{90}{CIFAR-100}}} 
                                                                             & \multirow{2}{*}{4-bit} & ResNet-18 & $ 73.60 \pm 0.98 $ & 69.02 & 74.17 \\
                                                                                                 &    & VGG-11& $ 60.04 \pm 4.30 $ & 43.20 & 67.35 \\\cline{2-6}
                                                                             & \multirow{2}{*}{8-bit} & ResNet-18  & $ 73.28 \pm 5.44 $ & 39.73 & 74.93 \\
                                                                                                 &    & VGG-11 & $ 60.38 \pm 4.57 $ & 50.46 & 68.21 
                                                                            \\\hline                                                                                       
    \end{tabular}}
    \vspace{3mm}
    \caption{Post attack accuracy T-BFA 1-to-1 stealthy}
\end{table*}

\begin{table*}[h]
    \centering
    \scalebox{1}{
    \begin{tabular}{|c|c|c|c|c|c|c|c|}\cline{3-8}
    \multicolumn{2}{c|}{} & \multicolumn{6}{c|}{Overhead - CPU cycles} \\\cline{3-8}
    \multicolumn{2}{c|}{} & \multicolumn{3}{c|}{4-bit precision} & \multicolumn{3}{c|}{8-bit precision} \\\hline
        Dataset & Model & $C_{(7,3)}$ & $C_{(8,4)}$ & $C_{(9,4)}$ & $C_{(12,3)}$ & $C_{(13,4)}$ & $C_{(14,4)}$ \\ \hline
        \multirow{2}{*}{CIFAR-10} & ResNet-20 & 39253976 & 39109892 & 45227044 & 43602516 & 44061354 & 44032176 \\
                                   & VGG-11 & 1683017718 & 1684937530 & 2001727596 & 1997017064 & 2017586802 & 2022746224 \\ \hline
        \multirow{2}{*}{CIFAR-100} & ResNet-18 & 1904310128 & 2034826394 & 2443498144 & 2265225840 & 2274760004 & 2293770526 \\
                                    & VGG-11 & 5222659354 & 5231379670 & 6129439010 & 6054743288 & 6105139016 & 6100082888 \\ \hline
    \end{tabular}}
    \vspace{3mm}
    \caption{Overhead in CPU cycles of decoding weights for quantized networks.}
    \label{tab:combined_overhead_cpu_cycles}
\end{table*}
